# Supplementary material for: Multi-dimensional parameter-space partitioning of spatio-temporal simulation ensembles
Source: arXiv:2205.00980 ancillary file (2022-05-03)
Supplement: Supplementary file 1 [file appendix.pdf]

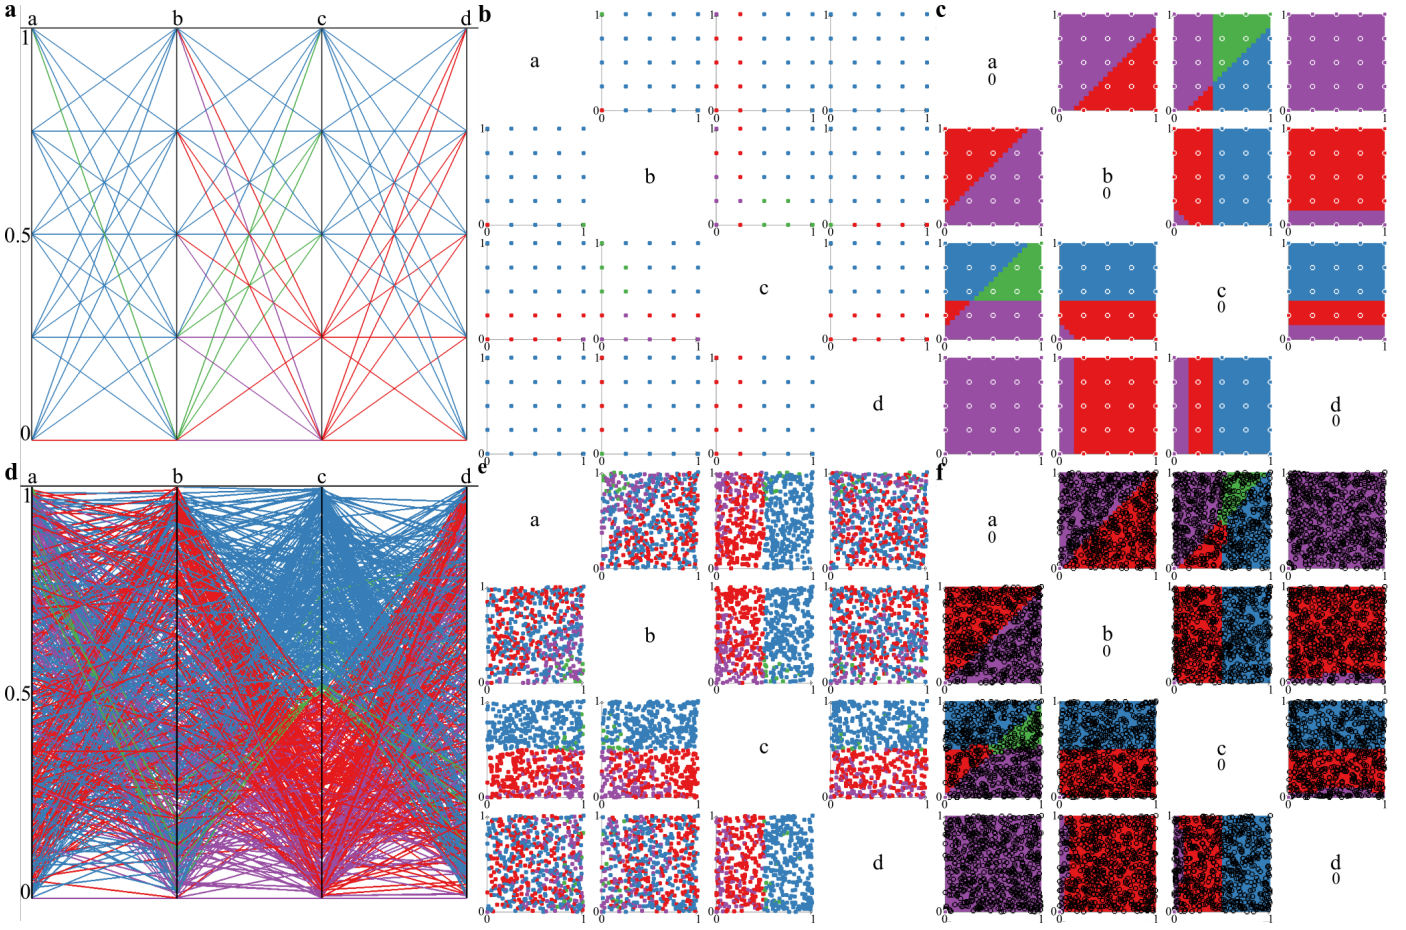

**Fig. 1.** Comparison for different parameter space visualization approaches. a, b, c) Structured sampling of parameter space. d, e, f) Monte Carlo sampling for parameter space. a) and d) show the parallel coordinates plot. b) and e) show the scatter plot matrix. c and f) show our hyper-slicer approach.

## 1. Synthetic Data

We use a synthetic dataset for the verification of our approach. For creating this dataset, we use four parameters ( $a$ - $d$ ) in the range of  $[0, 1]$  where parameter  $d$  does not influence the outcome. Thus, we analyze a four-dimensional parameter space. We sample this parameter space randomly using a Monte Carlo approach as well as on a structured grid. This allows a better comparison of the different approaches in Appendix 2. Note that we only use the structured version in the main article. For both cases, we create 625 samples in parameter space. Figure 2 (main article) shows the parameter space and one characteristic member of each region.

We create a 2D scalar field with a parameter-dependent number of Gaussians for each sample point in parameter space. The scalar field is defined over  $[0, 10] \times [0, 10]$  with a sampling of  $64 \times 64$ . One Gaussian in the center of the field is always present. Its standard deviation depends on the parameter  $a$ . The second Gaussian is located in the upper right corner of the field and is only present for  $c < 0.5$  and its standard deviation also depends on  $c$ . For the third Gaussian in the lower left corner with a standard deviation of 1, the parameter space is split on the diagonal of all relevant parameters. To differentiate the members, we add a small noise term where we use a uniform random noise with values between 0 and 0.1.

The three parameters  $a$ ,  $b$  and  $c$  divide the parameter space into four distinct regions with the following characteristics (the references refer to Figure 2 of the main article):

- 1) Only the Gaussian in the center (see Figure 2 I).
- 2) One Gaussian in the lower left corner and one in the center (see Figure 2 II).
- 3) One Gaussian in the upper right corner and one in the center (see Figure 2 III).
- 4) All three Gaussians (see Figure 2 IV).

The parameter space with the three relevant parameters is shown in Figure 2. The exact calculation for the scalar field  $g(\mathbf{x})$  is given as

$$g(\mathbf{x}) = \Theta(a - b - (1 - c)) \cdot f(\mathbf{x}; (1, 7), 1) \\ + \Theta(0.5 - c) \cdot f(\mathbf{x}; (9, 1), c + 1) \\ + f(\mathbf{x}; (5, 5), 0.1a + 1) + \zeta$$

where  $\zeta$  is uniform random noise in the range  $[0, 0.1]$ ,  $\Theta(z)$  is the Heavyside function with  $\Theta(z) = 0$  for  $z < 0$  and  $\Theta(z) = 1$  otherwise, and  $f(\mathbf{x}; (x_1, x_2), \sigma)$  is a 2D Gaussian kernel centered at  $(x_1, x_2)$  with standard deviation  $\sigma$ .

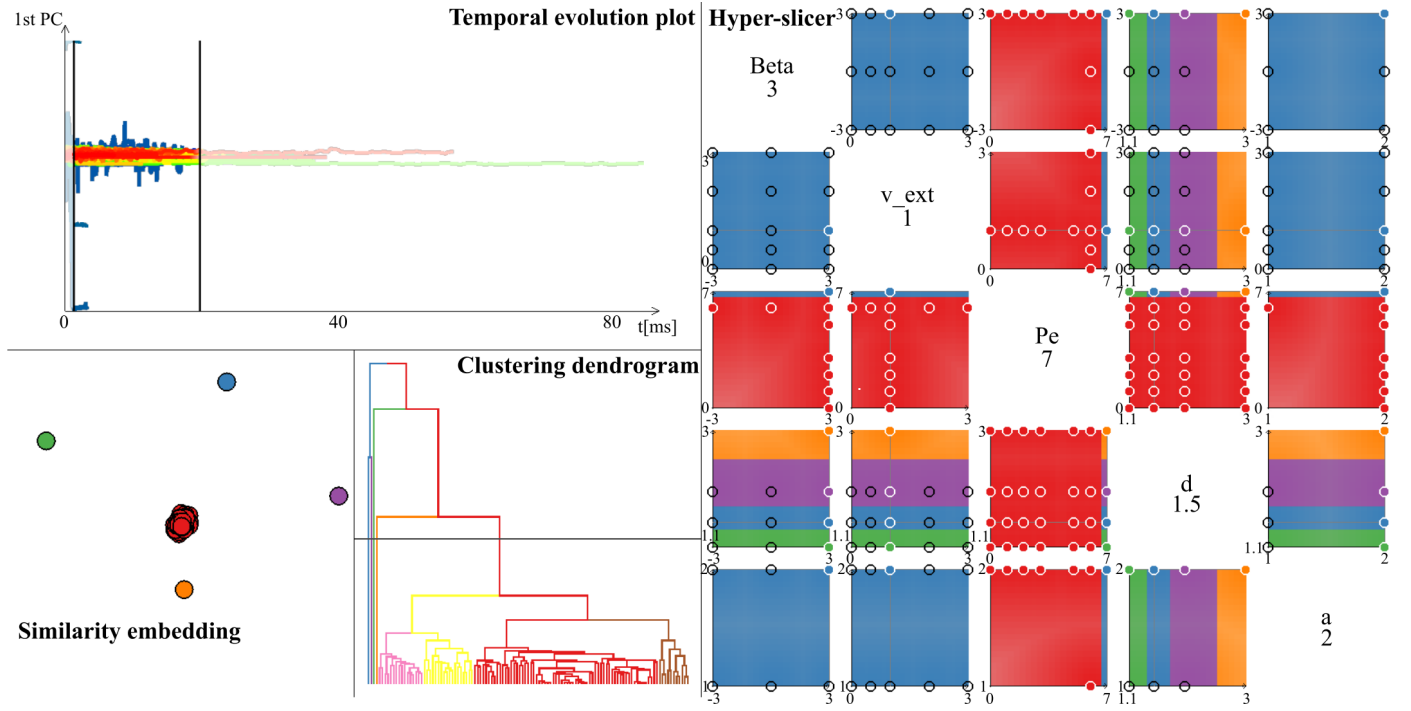

**Fig. 2.** Analysis of microswimmer dataset. The *temporal evolution plot* allows for selecting a temporal region of interest. Five similarity clusters can be observed in the *similarity embedding* and selected in the *clustering dendrogram*. The *hyper-slicer* allows us to investigate the induced parameter-space partitions.

## 2. Comparison to SPLOMs and PCPs

We compare our extended hyper-slicer approach to the use of scatter plot matrices (SPLOMs) and parallel coordinate plots (PCPs). Parameter spaces are often sampled on a structured grid, e.g., for the datasets presented in Section 7.1 (Bloodflow) and Appendix 3 (Microswimmers).

The results for a structured sampling of the parameter space are shown in Figure 1a-c. As in the hyper-slicer, the segments in the PCP and SPLOM are color-coded. One can directly see that both approaches suffer significantly from overplotting. The structured sampling can explain this. For PCP, it is especially problematic as all possible parameter combinations are present in the dataset. Thus, many lines are drawn on top of each other. This also explains why there are no visible purple lines between  $a$  and  $b$ . Another problem might arise due to misleading information. In both visualizations, it is not directly possible to see how many points or lines are drawn on top of each other. The visualization is also strongly impacted by the rendering order which determines which color is shown. Even though one can suspect from the PCP as well as the SPLOM that the red cluster only occurs for small values of  $c$  while the blue one is visible for larger values, it is not clear if this is not a projection artifact due to overplotting. The hyper-slicer itself does not directly solve this issue, but the projection of the cluster boundaries does solve this issue.

In principle, a similar extension can be introduced for PCP and SPLOM as well. However, the hyper-slicer enables the user to develop a geometric understanding. To compare the different approaches for this task, we use an unstructured sampling as presented in Figure 1d-f. In those cases, overplotting is less

prominent. However, it is still hard to identify some structures. For example, while the separation caused by parameter  $c$  can be identified in PCP and SPLOM, the diagonal structure for the green and the purple cluster is hardly visible (see Figure 2 in the main article for the shape of the segments in 3D). The local view of the hyper-slicer allows us to spot the diagonal shapes, for example, in the slice spanned by parameters  $a$  and  $c$ . The possibility to interactively change the focus point further supports building a geometric understanding of the parameter space (see video).

## 3. Case Study on Self-organization of Microswimmers

The simulations of this dataset aim at understanding the behavior of small swimmers, which can be, for example, bacteria or artificial particles. They are fixed in their positions but can rotate freely and interact with each other by the flow fields that they create. For our parameter-space segmentation, we used the pressure field created in a flow field simulation by using a finite element method. The simulation results depend on the shape of the particles which can be encoded in the aspect ratio, the distance between the particles, an external velocity applied to the system, the Péclet number (here on a logarithmic scale), and the propulsion mechanism, which is driven by the continuous numerical parameter  $\beta$ . The dataset consists of 115 runs with 18 to 308 adaptive timesteps. A spatial region of interest was resampled over a regular grid of size  $128 \times 128 \times 64$ .

To detect a temporal region of interest, we first analyzed the temporal evolution, see Figure 2. We observe a short transition phase at the beginning and a long time interval at the end where

1 most runs had already been terminated and not much is happen-  
2 ing for the others. Thus, we decided to only consider the time  
3 between 1.3 ms and 19.7 ms. Then, the distance matrix  $D_R$  was  
4 computed in 17.8 s.

5 Our approach proved to help identify interesting regions in  
6 parameter space, find clusters of similar runs, relate them to the  
7 corresponding parameter values, and understand outliers. We  
8 empirically decided to use *ward.D2* to create the hierarchical  
9 clustering, see Figure 2 for the clustering dendrogram. It was  
10 possible to identify four runs that strongly differ from the rest  
11 of the ensemble as can be seen in the similarity embedding in  
12 Figure 2. By investigating the parameter space, it becomes clear  
13 that these runs are located together in parameter space. They all  
14 have a parameter *beta* of 3 and an external velocity of 1. At the  
15 same time, they also share the same Péclet number and are all  
16 characterized by an aspect ratio *a* of 2. Thus, these simulation  
17 runs only differ in the distance between the particles.
